# Supplementary material for: VideoClusterNet: Self-Supervised and Adaptive Face Clustering For Videos
Source: arXiv:2407.12214 source file (2024-09-18)
Supplement: Supplementary file 1 [file appendix.tex]

\section{Implementation Details}

\subsection{Model Architecture}
\label{appendix:arch_details}
As part of our method, any CNN or Transformer architecture can be incorporated as the base Face ID model. For the attached MLP head, we incorporate a 3-layer network with GELU activation \cite{hendrycks2016_gaussian}. The length of the head's output feature embedding is kept the same as the base model's embedding length. Unnormalized model output embeddings are used for both training and the final clustering stage. Also, teacher branch head weights are initialized separately from their student counterpart. When using a transformer class base model, the head is shared between the class and path token embeddings in both student and teacher branches respectively (\cref{fig:ssl_finetuning}).

\subsection{Data Pre-Processing}
\label{appendix:data_preprocesing_details}
Generation of tracks as part of given video dataset curation for finetuning and/or clustering purposes involves processing the video through the four stage pipeline mentioned in detail in \cref{subsec:track_preprocessing}. To further augment variations in a sampled face crop pair, 'global' and 'local' views are created from the original crops. Specifically, crops are randomly resized and cropped with a scale between 0.7 and 1.0 to create multiple global crops, while a scale between 0.4 and 0.6 provides local crop variants.
Given a total of 6 views for each non-cropped original pair, we set the global and local crop count to 2 and 4 respectively.
%We set the global and local crop count to 2 and 4, for a total of 6 views for each base crop pair.
The loss for a given non-cropped original pair is computed using all possible pairs within each global and local crop group separately. We further apply horizontal flipping and color temperature variations as additional augmentations.  

Face alignment is performed for each face crop prior to the model finetuning and final clustering stages, in order to further enhance model learning of facial features and in turn for better face clustering performance. For this, a given face crop is first resized to the pre-trained model's expected input image size. Then, five point face landmarks are predicted for that crop (we incorporate the landmarks provided as an auxiliary output by the face detection model RetinaFace \cite{deng2020_retinaface} as we empirically find them to be quite accurate). Given the facial landmarks, a similarity transform is computed w.r.t. a mean landmark template. An affine warp is then computed to align the face within the face crop. 

\subsection{Model Finetuning}
\label{appendix:finetuning_details}
For the initial finetuning iteration, we train the model for 30 epochs. Note that the first 10 epochs are dedicated to finetuning the branch heads. All subsequent iterations include 10 training epochs without individual head training stages since the heads aren't randomly reinitialized for every new iteration. The teacher branch weights are updated with the exponential moving average of the student branch weights after every epoch. We adopt AdamW optimizer \cite{Loshchilov2019_decoupled} and an initial learning rate (lr) of $1 \times 10^{-4}$. We use cosine decay scheduling and reduce the lr to a final value of $1 \times 10^{-5}$. The initial lr is linearly warmed up for the first 5 epochs for each iteration from a starting value of $5 \times 10^{-6}$. Experiments were conducted using a Nvidia A10 GPU with 24 GB VRAM, running CUDA 12.0, with code implemented in PyTorch 1.13 \cite{Paszke2019_pytorch}. For finer details on the loss function and training hyperparameters, please refer to \cite{zhou2021_ibot}.

%\vspace{10px}
\subsection{Baseline Methods Implementation details}
\label{appendix:baseline_details}
\paragraph{Implementation for TSiam and SSiam \cite{sharma2019_self-supervised}} The methods were implemented in Pytorch 1.13 \cite{Paszke2019_pytorch}. For a fair comparison with other methods, we utilize ArcFace-R100 \cite{Jiankang2019_arcface} instead of VGGFace2 \cite{qiong2018_vggface2} as the base Face ID model. Since finer details on training hyperparameters are unavailable, we assume standard values for batch size (32 for TSiam) and training epochs (100). Besides, no image augmentations are added during training. We remark that we generate results on the MovieFaceCluster dataset tracks, excluding any bad face quality tracks that the original method struggles to cluster. A global threshold which was empirically deemed to be optimal for the entire MovieFaceCluster dataset was set as the cut-off threshold for HAC clustering module. For additional implementation details (which weren't modified in our implementation), please refer to \cite{sharma2019_self-supervised}.

\paragraph{Implementation for Joint Face Representation and Adaptation \cite{zhang2016_joint-face}} The approach was implemented in Pytorch 1.13 \cite{Paszke2019_pytorch}. For a fair comparison with other methods, we adopt ArcFace-R100 \cite{Jiankang2019_arcface} instead of DeepID2+ \cite{Sun2015_deeply} as the base Face ID model.
We implement a Markov Random Field (MRF) approach in Python from scratch for face clustering. For additional implementation details (which weren't modified in our implementation), please refer to \cite{zhang2016_joint-face}.
%Implementation for Markov Random Field (MRF) used for clustering was implemented in Python from scratch. 

%\vspace{10px}
\section{Additional details for track quality estimation}
\label{appendix:quality_estimation_details}
\paragraph{Threshold value for filtering out bad face quality tracks}
For a given set of $N$ tracks, a quality score threshold is computed as follows:
\begin{equation}
\label{equation:quality_score_threshold}
    thres(tqs(N)) = \overline{tqs(N)} - (2.7\times MAD(tqs(N))) 
\end{equation}
where $tqs(t_n)$ is the face quality score computed for the $n^{th}$ track using technique detailed in \cref{subsec:face_quality_estimation}, $tqs(N) = \{tqs(t_1),tqs(t_2),...,tqs(t_j)\} \hspace{0.1cm} \forall \hspace{0.1cm} j = \{1,2..,N\}$. Tracks having score lower than $thres(tqs(N))$ are filtered out from both coarse track matching and final clustering modules. The value of 2.7 was empirically found to work well for removing bad quality tracks from a wide range of movie track sets.

%\vspace{10px}
\section{Algorithm pseudo-code}
\label{appendix:algorithm_pseudo_code}
We present the pseudo-code of the different steps in our algorithm in \cref{alg:system_overview}. Mentioned stage numbers correspond to \cref{fig:system_overview}.

\begin{algorithm}[H] 
\SetCustomAlgoRuledWidth{0.45\textwidth}  
\scriptsize
\caption{VideoClusterNet}
  \textbf{Input:} \\
   \textbf{Face Tracks} $T=\{t_j | \hspace{0.1cm} j=1,2,...,N\}$ \\
    \hspace{0.5cm} $\ni t_j=\{I_{t_1},I_{t_2},...I_{t_n} | \hspace{0.1cm} f_{n+1}-f_n=12\}$ (obtained from stage 1)\\
   \textbf{pretrained model} $\theta_m$, \textbf{cluster iterations} $total \hspace{0.1cm} iters$ \\
    %\vspace{0.2cm}
    \textbf{Stage 2: Self Supervised model finetuning} \\
    $\theta_{s},\theta_{t} \longleftarrow \hspace{0.1cm} replicate(\theta_{m})$ \\
    $\theta_{s} \longleftarrow \hspace{0.1cm} \theta_{s} + attach \hspace{0.1cm} head(\theta_{h})$ \\ 
    $\theta_{t} \longleftarrow \hspace{0.1cm} \theta_{t} + attach \hspace{0.1cm} head(\theta_{h})$ \\ 
    $T_{filtered} = T, \hspace{0.1cm} T_{cm} = None$ \\
    %\vspace{0.1cm}
    \For{$i$ in $total \hspace{0.1cm} iters$}{
        $\theta_{s_{i}},\theta_{t_{i}} \longleftarrow \hspace{0.1cm} 
            finetune \hspace{0.1cm} model(\theta_{s_{i-1}},\theta_{t_{i-1}},T_{filtered}, T_{cm})$ \\
        $T_{fq} \longleftarrow \hspace{0.1cm} face \hspace{0.1cm} quality \hspace{0.1cm} estimation(T,\theta_{s_{i}}) $ \\
        $T_{filtered} \longleftarrow \hspace{0.1cm} filter \hspace{0.1cm} outliers(T,T_{fq}) $ \\ 
        $T_{cm} \longleftarrow \hspace{0.1cm} track \hspace{0.1cm} coarse \hspace{0.1cm} matching(\theta_{s_{i}}, T_{filtered}) $ \\ 
        $\theta_{ft} \longleftarrow \hspace{0.1cm} \theta_{s_{i}} $
    }
    %\vspace{0.2cm}
    \textbf{Stage 3: Fully Automated Face Track Clustering} \\
    $T_{fq} \longleftarrow \hspace{0.1cm} face \hspace{0.1cm} quality \hspace{0.1cm} estimation(T,\theta_{ft}) $ \\
    $T_{filtered} \longleftarrow \hspace{0.1cm} filter \hspace{0.1cm} outliers(T,T_{fq}) $ \\ 
    $C \longleftarrow \hspace{0.1cm} cluster \hspace{0.1cm} tracks(T_{filtered},\theta_{ft})$ \\
    %\vspace{0.2cm}
    \textbf{Output:} \textbf{Clustered track IDs} $C$ 
\label{alg:system_overview}
\end{algorithm}

%\vspace{10px}
\section{Additional results for BBT and BVS datasets}
\label{appendix:addi_BBT_BVS_results}
\begin{minipage}[c]{0.44\textwidth}
\scalebox{0.47}{
\begin{tabular}
{P{4.0cm}|P{0.7cm}|P{0.7cm}|P{0.7cm}|P{0.7cm}|P{0.7cm}|P{0.7cm}|P{1.4cm}}
 \textbf{Method} & \multicolumn{7}{|c}{\textbf{BBT Episode}} \\\cline{2-8}
        & S1E1 & S1E2 & S1E3 & S1E4 & S1E5 & S1E6 & Combined \\
 \hline
  \cite{wu2013_simultaneous-clustering} & 66.48 & - & - & - & - & - & - \\
  TSiam \cite{sharma2019_self-supervised} & 96.4 & - & - & - & - & - & - \\ 
  SSiam \cite{sharma2019_self-supervised} & 96.2 & - & - & - & - & - & - \\ 
  MLR \cite{bauml2013_semi-supervised} & 95.18 & 94.16 & 77.81 & 79.35 & 79.93 & 75.85 & 83.71 \\ 
  BCL \cite{tapaswi2019_video-face} & 98.63 & 98.54 & 90.61 & 86.95 & 89.12 & 81.07 & 89.63\\
  \hline \hline\rowcolor{LightCyan}
  Ours$\star$ & \textbf{99.70} & \textbf{99.67} & \textbf{98.60} & \textbf{98.80} & \textbf{99.10} & \textbf{97.10} & \textbf{98.70} \\\rowcolor{LightCyan}
  Ours$\dagger$ & 97.40 & 97.10 & 93.80 & 94.10 & 95.60 & 90.80 & 92.45 \\
\end{tabular}}
\captionof{table}{WCP/Clustering Accuracy on BBT Season 1. Here $\star$ / $\dagger$ denote not including / including filtered out tracks as an incorrect cluster, respectively. Note that we adopt ArcFace-R100 \cite{Jiankang2019_arcface} as our pre-trained base model.}
\label{table:BBT_addi_results}
\end{minipage}
\quad
\begin{minipage}[c]{0.53\textwidth}
\scalebox{0.49}{
\begin{tabular}{P{6.3cm}|P{0.7cm}|P{0.7cm}|P{0.7cm}|P{0.7cm}|P{0.7cm}|P{0.7cm}|P{1.2cm}}
 \textbf{Method} & \multicolumn{7}{|c}{\textbf{BVS Episode}} \\\cline{2-8}
        & S5E1 & S5E2 & S5E3 & S5E4 & S5E5 & S5E6 & Combined \\
 \hline
HMRF \cite{wu2013_constrained-clustering} & - & 50.3 & - & - & - & - & - \\
WBSLRR \cite{xiao2014_weighted-block} & - & 62.7 & - & - & - & - & - \\ 
TSiam \cite{sharma2019_self-supervised} & - & 92.46 & - & - & - & - & - \\ 
SSiam \cite{sharma2019_self-supervised} & - & 90.87 & - & - & - & - & - \\ 
CP-SSC \cite{somandepalli2019_reinforcing} & - & 65.2 & - & - & - & - & - \\
MvCorr \cite{somandepalli2021_robust} & - & 97.7 & - & - & - & - & - \\
MLR \cite{bauml2013_semi-supervised} & 71.99 & 61.27 & 66.60 & 67.07 & 69.59 & 61.72 & 66.37 \\ 
 BCL \cite{tapaswi2019_video-face}   & 92.08 & 79.76 & 84.00 & 84.97 & 89.05 & 80.58 & 83.62 \\\hline \hline \rowcolor{LightCyan}
  Ours$\star$ & \textbf{96.30} & \textbf{99.10} & \textbf{98.70} & \textbf{97.43} & \textbf{99.00} & \textbf{96.78} & \textbf{98.10} \\ \rowcolor{LightCyan}
  Ours$\dagger$ & 93.30 & 94.50 & 94.40 & 91.18 & 92.40 & 93.21 & 91.32 \\
\end{tabular}}
\captionof{table}{WCP/Clustering Accuracy on BVS Season 5. Here $\star$ / $\dagger$ denote not including / including filtered out tracks as an incorrect cluster, respectively. Note that we use ArcFace-R100 \cite{Jiankang2019_arcface} as our pre-trained base model.\looseness=-1}
\label{table:BVS_addi_results}
\end{minipage}

\section{MovieFaceCluster Dataset Curation}
\label{appendix:moviefacecluster_details}
The \textbf{MovieFaceCluster} dataset provides challenging face ID tracks within a set of hand-selected mainstream movies. These challenges involve large variations in pose, appearance, illumination and occlusions that are unavailable in any generic movie face ID datasets. To the best of our knowledge, this is the most comprehensive Video Face Identification dataset for movies to be open sourced. It consists of a total of 3619 face tracks across 209 different identities spanning nine movies. Each constituent movie has an unique set of characteristics in terms of number of characters, average track length, character age, ethnicity, and background environments, among other factors. Please refer to \cref{table:dataset_challenges} for further specific details on it.

%\vspace{0.5cm}
\scalebox{0.68}{
\begin{tabular}{P{6.5cm}|P{13.0cm}}
    \textbf{Movie / TV Series} & \textbf{Specific Face ID challenges} \\\hline\hline
    An Elephant's Journey (2019) & Bright outdoor scenes, American cast \\ \rowcolor{LightCyan}
    Armed Response & Low light scenes, facial occlusions with military helmets,sunglasses etc., African American and Middle Eastern Cast \\
    Angel Of The Skies & Unique heavy occlusions with oxygen masks in bright settings \\ \rowcolor{LightCyan} 
    Death Do Us Part (2019) & Low light scenes, Extreme facial expressions like screaming, Extreme poses, Rapid movements, African American Cast \\
    American Fright Fest & Facial occlusions like see through masks, sunglasses, extreme poses \\\rowcolor{LightCyan}
    The Fortress & Facial occlusions like headgear, Large main cast with primarily Asian characters  \\
    Under The Shadow & Low light scenes, Middle Eastern Cast\\ \rowcolor{LightCyan} 
    The Hidden Soldier & Low Light scenes, Asian Cast\\
    S.M.A.R.T. Chase & Extreme lighting in some scenes, Asian Cast\\\hline\hline \rowcolor{LightCyan} 
    Big Bang Theory (S1E01-06) & Mainly Indoor scenes in constant well lit environments, American cast\\ 
    Buffy The Vampire Slayer (S5E01-06) & Overall darker scenes, American Cast\\
    
\end{tabular}}
\captionof{table}{Specific Face ID challenges presented by each movie, as part of MovieFaceCluster dataset and literature benchmark datasets}
\label{table:dataset_challenges}

%\vspace{0.2cm}
Ground truth data is provided in form of tracks and face box spatial locations corresponding to a global movie frame index, w.r.t. a specific frame rate. These tracks are generated using the preprocessing module explained in detail in \cref{subsec:track_preprocessing}. As part of this processing stage, any bad quality tracks are discarded from the dataset. Also, each dataset movie consists of a mix of main and secondary characters. We remark that an unique face identity, which has at least two good quality tracks, is included as part of the movie dataset.

\section{Video Face Clustering Dataset Comparison}

In order to provide evidence to the uniqueness and advantages of our proposed MovieFaceCluster dataset compared to existing literature, in \cref{table:dataset_comparisons}, we present a comparison across some dataset attributes that are critical for the face clustering task. In \cref{fig:track_score_dist_comparison}, we present a dataset percent histogram comparison across face crop quality scores computed per dataset track using a large scale pretrained Face ID model (ArcFace-R100 \cite{Jiankang2019_arcface}). Similarly in \cref{fig:dataset_attribute_comparison}, we present a dataset percent histogram comparison for face crop parameters that are highly relevant for face clustering, namely scene lighting and face blur level. Scene lighting values are estimated as the average of lightness (L) parameter values in a given face crop image converted to HLS space. Face crop blur is estimated using a Singular Value Decomposition (SVD) based method \cite{su2011_blurred}. Significant differences weren't observed in face pose attribute across all datasets.

\begin{figure}[h]
\includegraphics[scale=0.8,width=12cm]{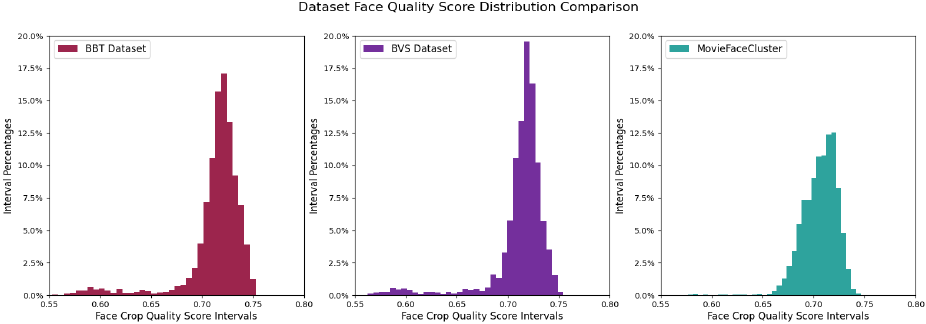}
\centering
\caption{Comparison of track face crop quality score distributions across The Big Bang Theory (BBT), Buffy, The Vampire Slayer (BVS) and our MovieFaceCluster dataset. For a given dataset, face crop quality score is computed for each of its constituent track. It is estimated as the average of scores calculated for a given track's sampled crop set (using SER-FIQ \cite{terhorst2020_ser-fiq} and  ArcFace-R100 \cite{Jiankang2019_arcface} as the pre-trained model for extracting embeddings). The distribution mean is relatively lower for our MovieFaceCluster dataset compared to other benchmark datasets, along with more bias towards lower quality score interval - 0.66 to 0.7. This provides empirical evidence towards our dataset containing more challenging cases for face clustering due to lower face quality scores.}
\label{fig:track_score_dist_comparison}
\end{figure}

\scalebox{0.68}{
\begin{tabular}{P{2.8cm}|P{3.5cm}|P{2.3cm}|P{2.2cm}|P{4.2cm}|P{2.5cm}}
     & & \multicolumn{4}{|c} {\textbf{Attribute}} \\\cline{3-6}
    \textbf{Dataset} & \textbf{TV series episode/Movie} & \textbf{Unique characters} & \textbf{Track Count} & \textbf{Unique ethnicity} (other than White/Caucasian) (cast percentage) & \textbf{Avg. Track Face Quality Score $\dagger \dagger$} \\\hline\hline
        & S01E01 & 6 & 647 & A (Minor) & 0.7193 \\
        & S01E02 & 5 & 613 & A (Minor) & 0.7108\\
    The Big Bang    & S01E03 & 7 & 562 & A (Minor) & 0.7094\\
    Theory (BBT)   & S01E04 & 8 & 568 & A (Minor) & 0.7140\\
        & S01E05 & 6 & 463 & A (Minor) & 0.7177\\
        & S01E06 & 6 & 651 & A (Minor) & 0.7111 \\\cline{3-6}
        &        & Average: 6.33 & Total: 3504 & Unique Count: 1 (A) & Average: 0.7136 \\\hline\hline
        & S05E01 & 12 & 786 & None & 0.7090 \\
        & S05E02 & 13 & 866 & None & 0.7117\\
Buffy The & S05E03 & 14 & 1185 & None & 0.7150\\
Vampire Slayer & S05E04 & 15 & 852 & None & 0.7125\\
  (BVS) & S05E05 & 15 & 733 & None & 0.7081\\
        & S05E06 & 18 & 1055 & None & 0.7142 \\\cline{3-6}
        &        & Average: 14.5 & Total: \textbf{5477} & Unique Count: 0 & Average: 0.7120 \\\hline\hline
        & An Elephant's Journey & 18 & 562 & None & 0.7112 \\
        & Armed Response & 14 & 119 & AA (Major), ME (Major) & 0.7085 \\
        & Angel Of The Skies & 29 & 319 & None & 0.7150\\
       & Death Do Us Part (2019) & 7 & 395 & AA (Major) & 0.7177 \\
 MovieFaceCluster        & American Fright Fest & 37 & 457 & AA (Minor) & 0.7098\\
        & The Fortress & 64 & 917 & A (Major) & 0.6918\\
        & Under The Shadow & 9 & 143 & ME (Major) & 0.7134\\
        & The Hidden Soldier & 21 & 594 & A (Major) & 0.7056\\
        & S.M.A.R.T. Chase & 10 & 113 & A (Major) & 0.7110\\\cline{3-6}
        &        & Average: \textbf{23.22} & Total: 3619 $\dagger$ & Unique Count: \textbf{3} (A,AA,ME) & Average: \textbf{0.7062}\\\hline

\end{tabular}}
\captionof{table}{Specific dataset attribute comparisons across BBT, BVS and our MovieFaceCluster dataset. A: Asian, AA: African American, ME: Middle Eastern characters. $\dagger$ Only tacks that contained decent quality face crops were added as part of each movie dataset. Bad face crop quality and background character tracks were discarded. $\dagger\dagger$ Score computed as average of all track crop quality scores as part of a given TV series episode/movie. A given track quality score is computed as average of quality scores for each of its sampled crops, using SER-FIQ \cite{terhorst2020_ser-fiq} and  ArcFace-R100 \cite{Jiankang2019_arcface} as the pre-trained model for extracting embeddings. A lower average quality score would mean that the given dataset contains on average more challenging cases for face clustering }
\label{table:dataset_comparisons}

\begin{figure}[h]
\includegraphics[scale=0.8,width=13cm]{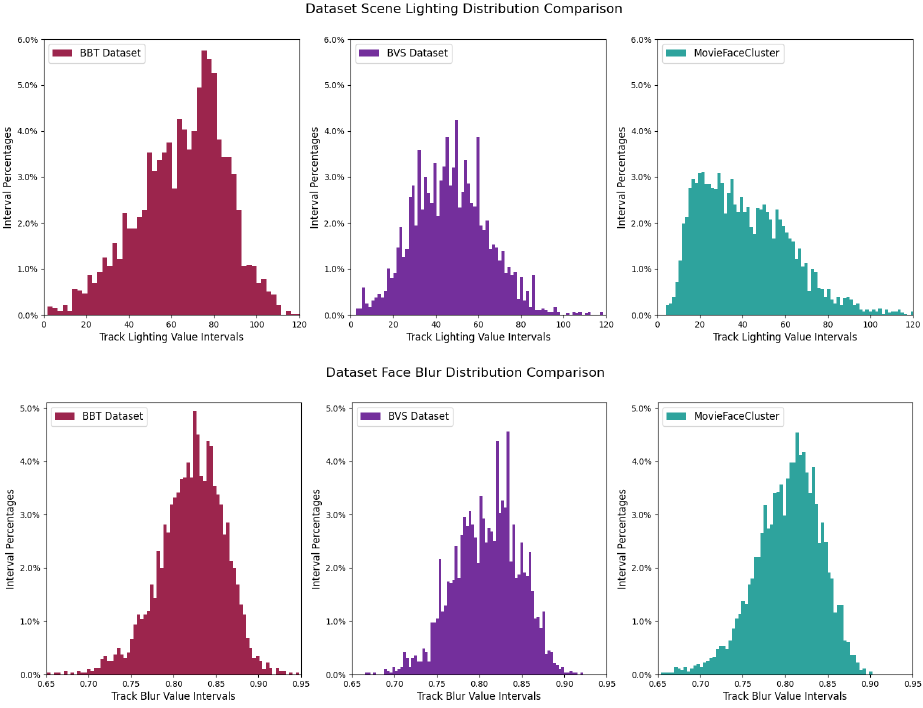}
\centering
\caption{Dataset attribute histogram comparisons for scene lighting and face bluriness across The Big Bang Theory (BBT), Buffy, The Vampire slayer (BVS) and our MovieFaceCluster dataset. Each respective dataset attribute is computed per track, taken as average of each of its sampled crops attributes. For Scene Lighting,  MovieFaceCluster has higher distribution variance compared to literature datasets, with more bias towards darker lighting (values have positive correlation to amount of track scene lighting). For Face Blur, MovieFaceCluster has higher sample count in 0.65 to 0.75 value range compared to literature datasets, providing evidence of having higher level of bluriness in track face crops (Blur values have negative correlation to amount of blur present in face crops).}
\label{fig:dataset_attribute_comparison}
\end{figure}

With reference to \cref{table:dataset_comparisons}, our proposed MovieFaceCluster dataset has on average lot more unique character faces and significantly better cast racial diversity. Also, it manages to obtain a much lower average face quality score, alluding to the fact that our dataset contains on average more challenging data samples w.r.t. face clustering/identification task. \cref{fig:track_score_dist_comparison} further strengthens this argument by providing evidence of higher percent of dataset tracks having lower face quality scores within our dataset. In addition, \cref{fig:dataset_attribute_comparison} signifies, firstly that MovieFaceCluster has higher variance in scene lighting across its face samples with bias towards lot darker scenes which helps provide harder scenarios for face clustering. Secondly, for facial blur, our dataset has higher count of track samples with larger amount of facial blur compared to literature datasets, which again helps provide more challenging scenarios for face clustering.  

%\vspace{0.7cm}
\section{Training and evaluation timings}
\label{appendix:timing_evaluation}
Our proposed algorithm comprises two main stages from a computation standpoint: 1) Model SSL finetuning and 2) Final clustering. \cref{table:method_timings} presents run times of each of these stages for each movie of \textbf{MovieFaceCluster} dataset.  

%\vspace{0.3cm}
\scalebox{0.55}{
\begin{tabular}{P{3.6cm}|P{1.9cm}|P{1.7cm}|P{1.7cm}|P{1.7cm}|P{1.7cm}|P{1.5cm}|P{1.7cm}|P{1.7cm}|P{1.7cm}|P{1.7cm}}
            & \multicolumn{10}{|c}{\textbf{Movie}} \\\cline{2-11}
 \textbf{Statistics} &  An &  Armed & Angel & Death & American & The & Under & The & S.M.A.R.T. & Average \\
            & Elephant's & Response & Of The &  Do Us &  Fright &  Fortress &  The & Hidden & Chase & (Per \\
            & Journey(2019) & & Skies &  Part (2019) & Fest  &  & Shadow & Soldier & & Track) \\\hline 
Track Count & 562 & 119 & 319 & 395 & 457 & 917 & 143 & 594 & 113 & - \\\rowcolor{LightOrange}
Finetuning Iterations & 5 & 6 & 5 & 8 & 10 & 9 & 6 & 5 & 5 & - \\
Model Finetuning (mins) & 193.76 & 38.45 & 110.16 & 397.24 & 298.41 & 645.06 & 57.21 & 307.12 & 48.19 & 0.579 \\ \rowcolor{LightOrange}
Final Clustering (secs) & 66.36 & 6.74 & 28.42 & 40.82 & 61.94 & 167.32 & 13.93 & 81.32 & 9.13 & 0.132 \\\hline

\end{tabular}}
\captionof{table}{Training iteration count and runtimes for SSL finetuning and final clustering computed on MovieFaceCluster dataset. Here, the training iteration count represents the SSL finetuning iteration at which the process was terminated, and final clustering was performed.}
\label{table:method_timings}

%\vspace{0.7cm}
\section{SSL finetuning iteration ablation}
\label{appendix:iteration_ablation}
\begin{wrapfigure}[13]{R}{0.45\textwidth} 
%\vspace{-0.4cm}
\scalebox{0.64}{
\begin{tabular}{P{2.4cm}|P{2.7cm}|P{3.2cm}}
 \textbf{SSL Finetuning} & \textbf{Accuracy / WCP} & \textbf{Pred Cluster Ratio/}\\
\textbf{ Iteration} & \textbf{(\%)} & \textbf{PCR (Pred / GT)} \\\hline\hline 
1 & 52.56 & 0.476 (10/21) \\
2 & 72.12 & 0.571 (12/21) \\ 
3 & 91.38 & 1.114 (24/21) \\
4 & 96.93 & 1.000 (21/21) \\\rowcolor{LightCyan}
\textbf{5} & \textbf{99.50} & \textbf{1.048 (22/21)} \\
6 & 99.41 & 1.095 (23/21) \\ 
7 & 99.47 & 1.095 (23/21) \\
8 & 99.50 & 1.190 (25/21) \\ 
9 & 99.50 & 1.238 (26/21) \\ 
10 & 99.41 & 1.238 (26/21) \\\hline
\end{tabular}}
\captionof{table}{Ablation for SSL finetuning iterations parameter, presented for \textbf{MovieFaceCluster:The Hidden Soldier} dataset. Finetuning until iteration 5 provides optimal results in terms of both metrics.}
\label{table:ablation_ssl_iterations}
\end{wrapfigure}

This section provides ablation results for the Self-Supervised Learning (SSL) finetuning iteration parameter, performed on the MovieFaceCluster:The Hidden Soldier dataset. Our overall experiments showed that a minimum of 5 iterations are required to obtain optimal results. Additional few iterations (e.g., 2 or 3) are necessary for harder datasets. This is assuming the first iteration is run for about 30 epochs, with each succeeding one comprising 10 epochs. For iteration 10 and above, our method might over-cluster the dataset, i.e., it finds sub-clusters within the optimal clusters, optimizing for variants of a given character. Note that the first SSL finetuning iteration involves image pair generation from within the same track only. For all succeeding iterations, image pairs are generated across coarse-matched tracks, facilitated through the coarse track matching process detailed in \cref{subsec:track_matching}.  

\clearpage
\section{Additional t-SNE visualizations}
\label{appendix:addi_t_sne_viz}
\cref{fig:addi_viz_1,fig:addi_viz_2,fig:addi_viz_3} present additional t-SNE learned embedding visualizations for select movies that are part of the \textbf{MovieFaceCluster} dataset.  

\begin{figure}[h]
\includegraphics[scale=0.8,width=14cm]{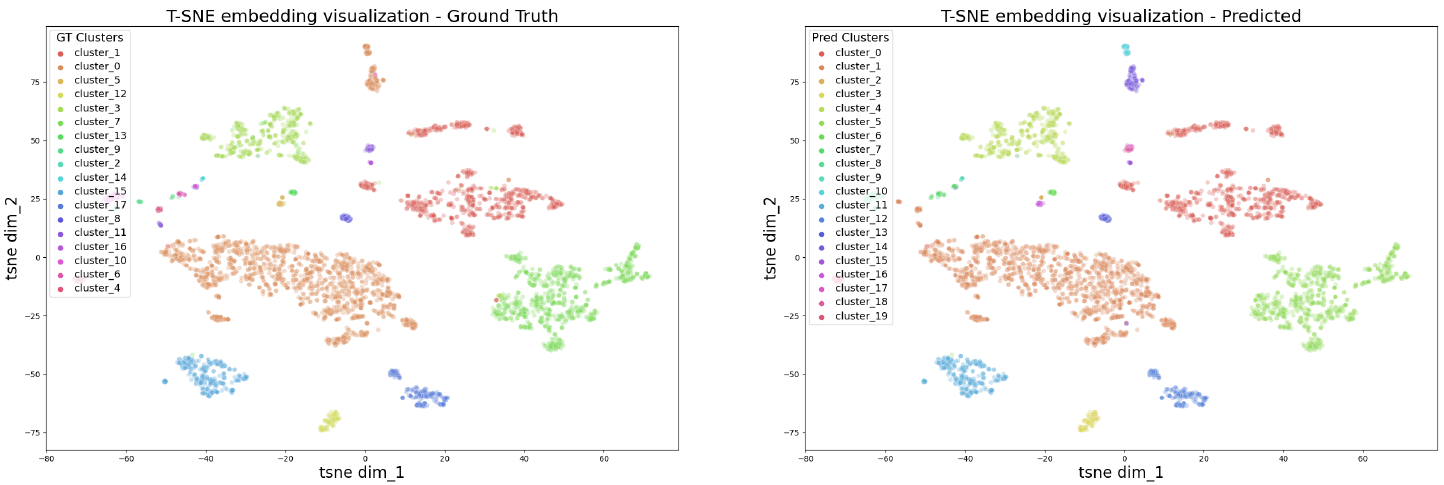}
\centering
\caption{Comparative t-SNE embedding visualizations on \textbf{MovieFaceCluster:An Elephant's Journey} dataset. \textit{Left:} Ground truth, \textit{Right:} Our method. Each dot in the diagram above represents the finetuned model's extracted embedding for a face crop $I_{t_{n}}$ in a given track's sampled crop set $t$. Face embeddings assigned to a given color constitute a single cluster.}
\label{fig:addi_viz_1}
\end{figure}

\begin{figure}[h]
\includegraphics[scale=0.8,width=14cm]{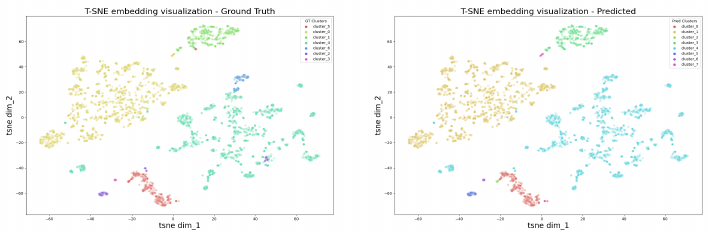}
\centering
\caption{Comparative t-SNE embedding visualizations on \textbf{MovieFaceCluster:Death Do Us Part} dataset. \textit{Left:} Ground truth, \textit{Right:} Our method. Each dot in the diagram above represents the finetuned model's extracted embedding for a face crop $I_{t_{n}}$ in a given track's sampled crop set $t$. Face embeddings assigned to a given color constitute a single cluster.}
\label{fig:addi_viz_2}
\end{figure}

\begin{figure}[h]
\includegraphics[scale=0.8,width=14cm]{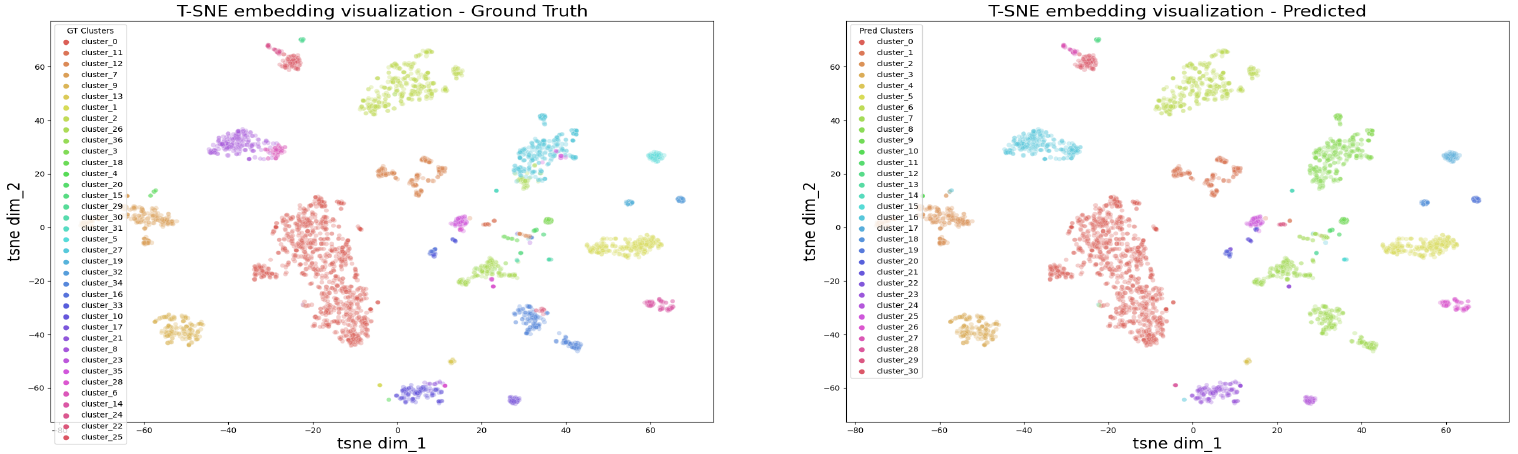}
\centering
\caption{Comparative t-SNE embedding visualizations on \textbf{MovieFaceCluster:American Fright Fest} dataset. \textit{Left:} Ground truth, \textit{Right:} Our method. Each dot in the diagram above represents the finetuned model's extracted embedding for a face crop $I_{t_{n}}$ in a given track's sampled crop set $t$. Face embeddings assigned to a given color constitute a single cluster.}
\label{fig:addi_viz_3}
\end{figure}

\clearpage
\section{Additional hard case cluster visualizations}
\label{appendix:addi_hard_case_viz}
\cref{fig:addi_hard_case_viz} presents an additional selection of hard case cluster results obtained with our proposed method on the \textbf{MovieFaceCluster} dataset.

\begin{figure}[H]
\includegraphics[scale=0.8,width=13cm]{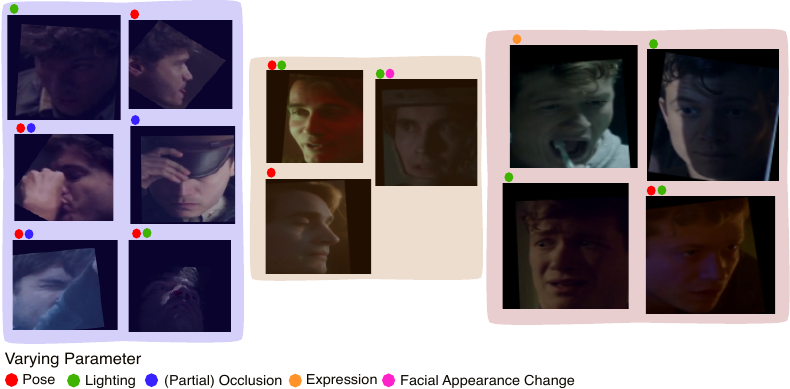}
\centering
\caption{Select hard case clusters obtained through our proposed method on \textbf{MovieFaceCluster} dataset. The term “varying parameter” depicts the dominant image attributes that are particularly challenging for a given face crop. It isn’t part of the available dataset annotations but simply mentioned for enhanced reader understanding.} 
\label{fig:addi_hard_case_viz}
\end{figure}

% {\small
% \bibliographystyle{iclr2024_conference}
% \bibliography{00.main}
% }

% \end{document}
